# Supplementary material for: xCoT: Cross-lingual Instruction Tuning for Cross-lingual Chain-of-Thought Reasoning
Source: arXiv:2401.07037 source file (2024-01-13)
Supplement: Supplementary file 1 [file Appendix.tex]

\appendix

\appendix
\section{Statistics of Datasets}
% \paragraph{Bilingual Translation} For the bilingual task, we use the \textbf{WMT-14 English-German}, \textbf{WMT-14 English French}, and \textbf{WMT-16 English-Romanian} benchmark for evaluation. 
% WMT-14 En-De from WMT consists of 4.5M sentence pairs. The valid set is newstest2013 and the test set is newstest2014. WMT-14 En-Fr is a large-scale dataset containing nearly 41M sentence pairs and newstest2014 is employed for evaluation.
% WMT-16 En-Ro is comprised of original parallel sentences and back-translation data. 
%We use newsdev2016 for validation and newstest2016 for test.

\paragraph{WMT-14 En-De} WMT-14 En-De consists of 4.5M sentence pairs. The validation set is devtest2014, and the test set is newstest2014.\footnote{\url{https://statmt.org/wmt14/translation-task.html}}

\paragraph{WMT-16 En-Fr} WMT-14 En-Fr is a large-scale dataset containing nearly 41M sentence pairs, where newstest2014 is employed for evaluation.

\paragraph{WMT-16 En-Ro} WMT-16 En-Ro is comprised of original parallel sentences and back-translation data. We use newsdev2016 for validation and newstest2016 for test. Following the previous work \cite{mbart}, we use the same back-translation data for a fair comparison.\footnote{\url{https://www.statmt.org/wmt16/translation-task.html}}

\paragraph{IWSLT-2017} We download English (En), German (De), Italian (It), Dutch (Nl), and Romanian (Ro) corpora from the IWSLT-2017 benchmark. The dev2010 is used for validation and tst2017 for test.\footnote{\url{https://sites.google.com/site/iwsltevaluation2017/TED-tasks}}

\paragraph{WMT-10} Table~\ref{tab:wmt10} lists the detailed statistics of 10 language pairs from WMT-10, which is a collection of parallel data in different languages from the WMT datasets.
The parallel data is paired with English and other 10 languages, including French (Fr), Czech (Cs), German (De), Finnish (Fi), Latvian (Lv), Estonian (Et), Romanian (Ro), Hindi (Hi), Turkish (Tr) and Gujarati (Gu). The corpora of the WMT benchmark, exclude WikiTiles, from the latest available year of each language are chosen. After removing the duplicated samples, we limit the size of each parallel language pair data up to 10 million by randomly sampling from the whole corpus. We adopt the same valid and test sets from the WMT benchmark as the previous work \cite{zcode}.

\paragraph{WikiLingua} To test the capability of our multilingual pre-trained model, a large-scale multilingual dataset named \textbf{WikiLingua} \cite{wikilingua} of 18 languages from WikiHow is used to evaluate multilingual abstractive summarization systems.\footnote{\url{https://github.com/esdurmus/Wikilingua}}

%%%%%%%%%%%%%%%%%%%%%%%%%%%%%%%%%%%%%%%%%%%%%%%%%%%%%%%
\begin{table}[htb]
\centering
\resizebox{1.0\columnwidth}{!}{
\begin{tabular}{ccccccc}
\toprule
Code & Language & \#Bitext & Training & Valid & Test \\
\midrule
Fr & French & 10M     & WMT15 & Newstest13 & Newstest15 \\
Cs & Czech & 10M      & WMT19 & Newstest16 & Newstest18 \\
De & German & 4.6M    & WMT19 & Newstest16 & Newstest18 \\
Fi & Finnish & 4.8M   & WMT19 & Newstest16 & Newstest18 \\
Lv & Latvian & 1.4M   & WMT17 & Newsdev17 & Newstest17 \\
Et & Estonian & 0.7M  & WMT18 & Newsdev18 & Newstest18 \\
Ro & Romanian & 0.5M  & WMT16 & Newsdev16 & Newstest16 \\
Hi & Hindi & 0.26M    & WMT14 & Newsdev14 & Newstest14 \\
Tr & Turkish & 0.18M  & WMT18 & Newstest16 & Newstest18 \\
Gu & Gujarati & 0.08M & WMT19 & Newsdev19 & Newstest19 \\
\bottomrule
\end{tabular}}
\caption{Statistics and sources of the training, valid, and test sets from WMT between English and other languages.}
\vspace{-10pt}
\label{tab:wmt10}
\end{table}
%%%%%%%%%%%%%%%%%%%%%%%%%%%%%%%%%%%%%%%%%%%%%%%%%%%%%%%

\section{Pre-training and Fine-tuning Details}
\paragraph{Pre-training Hyper-parameters} Table \ref{tab:pretraining_hyperparams} summarizes the hyper-parameters for pre-training \ourmethod{} and \mourmethod{}
The task-specific hyper-parameters for the downstream language generation and understanding tasks are in Table \ref{tab:task_specific_hyperparams}. 

\paragraph{Abstractive Summarization} 
During fine-tuning, we use the Adam \cite{adam} optimizer with an initial learning rate of 1e-4 and the batch size is set as 2048 tokens on 8 V100 GPUs. The models
are trained with the label smoothing cross-entropy with a smoothing ratio of 0.1. The last 5 checkpoints are averaged for evaluation. 

%To mitigate the unbalance of the multilingual corpora, \cite{mnmt_challenges,zcode}, we employ the temperature-based sampling method for all multilingual experiments, where the peak temperature is set as $\tau_{1} = 5.0$ to sample more pairs in low-resource languages. We use the same sampling strategy for all multilingual tasks.
\paragraph{Neural Machine Translation} We adopt Adam with a learning rate of 1e-4 and set the batch size as 2048 tokens on 8 V100 GPUs for all bilingual translation tasks and the IWSLT-2017 benchmark. For the large-scale multilingual dataset WMT-10, our pre-trained model is fine-tuned on 32 V100 GPUs with a learning rate of 3e-4. For a fair comparison, we adopt the same architecture and model size as our pre-trained model.
\paragraph{Data-to-text Generation} 
We use Adam with a learning rate of \{8e-5,1e-4\} and set the batch size as 16 sentences on the WebNLG dataset.

\paragraph{Multi-lingual Fine-tuning} Following the previous work~\cite{zcode,deltalm}, we adopt a dynamic temperate-based sampling strategy to mitigate the unbalance of the multilingual corpora, where we gradually sample more pairs in low-resource languages with the number of epochs increasing. The temperature of the $i$-th epoch is calculated by:
\begin{equation}
\begin{MiddleEquation}
    \tau_{i}=\min(\tau_{1}, \tau_{0}+\frac{i}{N}(\tau-\tau_{0}))
    \label{epoch_temperature}
\end{MiddleEquation}
\end{equation}
where $\tau_{0}$ is the initial temperature, $\tau_{1}$ is the peak temperature, and $N$ is the number of warm-up epochs. We set $\tau_{0}=1.0$, $\tau_{1}=5.0$, and $N=5$ for all multilingual experiments for a fair comparison. 

Given the temperature $\tau_{i}$ $i$-th epoch, we can calculate the real sampling ratio of the language $L_{k}$, where $L_{k} \in L_{all}=\{L_{1},\dots,L_{K}\}$:
\begin{equation}
\begin{MiddleEquation}
    q_{L_{k}}(i)=\frac{p_{L_{k}}^{\frac{1}{\tau_{i}}}}{\sum_{j=1}^{K} p_{L_{j}}^{\frac{1}{\tau_{i}}}}
\end{MiddleEquation}
\end{equation}
where $q_{L_{k}}(i)$ is the sampling ratio of the language $L_k$ in the $i$-th epoch. $p_{L_k}$ is the real data ratio of the language $L_{k}$ in all languages. $\tau_{i}$ is the temperature of the $i$-th epoch, as described in Equation \ref{epoch_temperature}.

\begin{table}[t]
\begin{center}
\resizebox{1.0\columnwidth}{!}{
\begin{tabular}{lccc}
\toprule
\bf Hyper-parameter  & \bf \ourmethod{} & \bf \mourmethod{} \\
\midrule 
Number of Encoder Layers             & 12 & 12 \\
Number of Generator Layers           & 12 & 12 \\
Number of Discriminator Layers       & 4 & 4 \\
Hidden size                          & 768 & 768 \\
FFN hidden size                      & 3072 & 3072 \\
Attention heads        & 12 & 12 \\
Attention head size    & 64 & 64 \\
Dropout                & 0.1 & 0.1 \\
Attention Dropout      & 0.1 & 0.1 \\
Warmup Steps           & 10k & 10k \\
Peak Learning Rate     & 4e-4 & 5e-4 \\
Batch Size             & 8K & 8K \\
Weight Decay           & 0.01 & 0.01 \\
Max Steps              & 500k & 500k\\
Learning Rate Decay    & Linear & Linear \\
Adam $\beta_1$         & 0.9 & 0.9 \\
Adam $\beta_2$         & 0.98 & 0.98 \\
Gradient Clipping      & 0.0 & 0.0 \\
\bottomrule
\end{tabular}}
\end{center}
\caption{Hyper-parameters for pre-training \ourmethod{} and \mourmethod{}.}
\label{tab:pretraining_hyperparams}
\end{table}

\begin{table*}[htb]
\resizebox{1.0\textwidth}{!}{
\centering
\begin{tabular}{lccccccccc}
\toprule
\bf Task &\bf Learning Rate & \bf Warmup Steps & \bf Batch Size  & \bf Weight Decay & \bf Max Epoch & \bf Gradient Clipping & \bf \makecell[c]{Max Source Positions} & \bf \makecell[c]{Max Target Positions} \\
\midrule
\multicolumn{6}{l}{\textit{Text Summarization}} \\
\midrule
CNN / DailyMail & 1e-4 & 1000  & 2048 (Tokens) & 0.0 & 16 & 0.0 & 608 & 160  \\
XSum            & 1e-4 & 1000  & 2048 (Tokens) & 0.0 & 16 & 0.0 & 720 & 48 \\
WikiLingua     & 1e-4 & 1000  & 2048 (Tokens) & 0.0 & 16 & 0.0 & 512 & 160 \\
\midrule
\multicolumn{6}{l}{\textit{Machine Translation}} \\
\midrule
WMT14 En-De     & 1e-4 & 4000  & 2048 (Tokens) & 0.0 & 50  & 0.0 & 512 & 512\\
WMT14 En-Fr     & 1e-4 & 4000  & 2048 (Tokens) & 0.0 & 50  & 0.0 & 512 & 512\\
WMT14 En-Ro     & 1e-4 & 4000  & 2048 (Tokens) & 0.0 & 16  & 0.0 & 512 & 512\\
IWSLT17         & 1e-4  & 4000  & 2048 (Tokens) & 0.05 & 16 & 0.0 & 512 & 512 \\
WMT10           & 3e-4  & 4000  & 2048 (Tokens) & 0.0 & 8  & 0.0 & 512 & 512 \\
\midrule
\multicolumn{6}{l}{\textit{Data-to-Text}} \\
\midrule
WebNLG          & \{2.5e-5, 5e-5\}  & 1000  & 2048 (Tokens) & 0.05 & 16 & 0.0 & 512 & 512 \\
\midrule
\multicolumn{6}{l}{\textit{Natural Language Understanding}} \\
\midrule
XNLI          & \{2.5e-5, 5e-5\}  & 4000  & 16 (Sentences) & 0.05 & 30 & 1.0 & 512 & 512 \\
GLUE          & \{1e-5, 2.5e-5, 5e-5\}  & 4000  & \{8,16\} (Sentences) & 0.05 & 30 & 1.0 & 512 & 512 \\
\bottomrule
\end{tabular}
}
\caption{
Task-specific hyper-parameters for downstream language generation and understanding benchmarks.
}
\label{tab:task_specific_hyperparams}
\end{table*}

%%%%%%%%%%%%%%%%%%%%%%%%%%%%%%%%%%%%%%%%%%%%%%%%%%%%%%%%%%%%%%%%%%%%%%%%%%%%%%%%%%%%%%%%%%%%%%%%%%%%%%%
\section{Results on Downstream Task}
\paragraph{GLUE} For each classification task of the GLUE \cite{glue}, we conduct 5 experiments with different seeds $\{1,2,3,4,5\}$ and report the average accuracy of 5 experiments.

\paragraph{XNLI} We also conduct 5 experiments with different seeds $\{1,2,3,4,5\}$ and report the average accuracy of 5 experiments.

\paragraph{FLORES} Since the corpora of $X \to Y$ are commonly scarce, the performance of low-resource translation direction Avg$_{X \to Y}$ mainly depends on the zero-shot cross-lingual transferability of the pre-trained model. Our model with the 12 encoder layers and 12 decoder layers significantly outperforms the previous state-of-the-art model M2M-124 with large model size.
In Figure \ref{flores_all}, we report the multilingual model initialized by our pre-trained model in all translation directions, where the languages are ordered alphabetically by the language code.
Following the previous work \cite{microsoft_wmt2021}, we use the same training data, including CCAligned \cite{ccalign}, CCMatrix \cite{ccmatrix}, OPUS-100 \cite{opus_100}, JW300 \cite{jw300}, Tatoeba \cite{tatoeba}, WMT2021 news track\footnote{\url{http://statmt.org/wmt21/translation-task.html}}, multilingual track data\footnote{\url{http://data.statmt.org/wmt21/multilingual-task/}}.
%%%%%%%%%%%%%%%%%%%%%%%%%%%%%%%%%%%%%%%%%%%%%%%%%%%%%%%%%%%%%%%%%%%%%%%%%%%%%%%%%%%%%%%%%%%%%%%%%%%%%%%%%%%%%%%%%%%%%%%%%%%%
\begin{table}[t]
\centering
\resizebox{0.9\columnwidth}{!}{
\begin{tabular}{lccccccc}
\toprule
 \bf Seed     & \bf MNLI & \bf SST-2 & \bf MRPC & \bf RTE & \bf QNLI  & \bf QQP & \bf Avg$_{\bm{6}}$ \\ \midrule
\multicolumn{8}{l}{\textit{Fine-tuning on Discriminator ($\mathcal{D}$)}}    \\
 \midrule
1        & 88.9   & 94.5  & 89.7  & 83.8   & 93.8  & 91.6     & 90.4     \\
2        & 89.1   & 94.7  & 90.0  & 84.8   & 93.9  & 91.7     & 90.7     \\
3        & 88.9   & 94.5  & 91.7  & 83.0   & 93.7  & 91.9     & 90.6     \\
4        & 89.0   & 94.7  & 90.9  & 84.1   & 93.8  & 91.8     & 90.7     \\
5        & 89.2   & 95.2  & 90.7  & 80.1   & 94.2  & 91.7     & 90.2     \\
Avg      & 89.0   & 94.7  & 90.6  & 83.2   & 93.9  & 91.7     & 90.5     \\
 \midrule
\multicolumn{8}{l}{\textit{Fine-tuning on Generator ($\mathcal{G}$)}} \\
 \midrule
1       & 89.2   & 95.1   & 90.4  & 85.6   & 94.1  & 91.9     & 91.0    \\
2       & 89.1   & 95.2   & 90.9  & 85.6   & 94.3  & 92.1     & 91.2    \\
3       & 89.2   & 95.0   & 90.4  & 84.5   & 94.1  & 91.9     & 90.9    \\
4       & 89.4   & 95.1   & 90.9  & 84.8   & 94.1  & 92.1     & 91.1    \\
5       & 89.6   & 94.8   & 89.7  & 84.5   & 94.2  & 91.8     & 90.8    \\
Avg     & 89.3   & 95.0   & 90.5  & 85.0   & 94.2  & 92.0     & 91.0    \\
\bottomrule
\end{tabular}}
\caption{The accuracy scores of the base-setting models on the valid set of GLUE classification tasks.}
\label{tab:glue_seed}
\vspace{-10pt}
\end{table}
%%%%%%%%%%%%%%%%%%%%%%%%%%%%%%%%%%%%%%%%%%%%%%%%%%%%%%%%%%%%%%%%%%%%%%%%%%%%%%%%%%%%%%%%%%%%%%%%%%%%%%%%%%%%%%%%%%%%%%%%%%%%%%%%%%

%%%%%%%%%%%%%%%%%%%%%%%%%%%%%%%%%%%%%%%%%%%%%%%%%%%%%%%%%%%%%%%%%%%%%%%%%%%%%%%%%%%%%%
\begin{table*}[htb]
\centering
\resizebox{1.0\textwidth}{!}{
\begin{tabular}{l|ccccccccccccccc|c}
\toprule
\bf Model & \bf En & \bf Ar & \bf Bg & \bf De & \bf El & \bf Es & \bf Fr & \bf Hi & \bf Ru & \bf Sw & \bf Th & \bf Tr & \bf Ur & \bf Vi & \bf Zh & \bf Avg$_{\bm{15}}$ \\
\midrule
\multicolumn{17}{l}{\emph{Cross-lingual zero-shot transfer (models fine-tune on English data only)}} \\
\midrule

mBERT     & 80.8 & 64.3& 68.0& 70.0& 65.3& 73.5& 73.4& 58.9& 67.8& 49.7& 54.1& 60.9& 57.2& 69.3& 67.8& 65.4 \\
XLM       & 85.0 & 73.1 & 77.4 & 77.8 & 76.6  & 78.9 & 78.7 & 69.6 & 75.3 & 68.4 & 73.2 & 72.5 &67.3 &76.1 &76.5 & 75.1\\
mT5-Small & 79.6 & 65.2 & 71.3 & 69.2 & 68.6  & 72.7 & 70.7 & 62.5 & 70.1 & 59.7 & 66.3 & 64.4 &59.9 &66.3 & 65.8 & 67.5 \\
mT5-Base  & 84.7 & 73.3 & 78.6 & 77.4 & 77.1  & 80.3 & 79.1 & 70.8 & 77.1 & 69.4 & 73.2 & 72.8 & 68.3 & 74.2 & 74.1 & 75.4 \\
\mourmethod{} (D) &     85.9 &     72.6 & \bf 78.6 &     78.6 & \bf 76.6 & \bf 80.7 &     79.8 &     70.4 &     76.0 & \bf 64.4 & \bf 74.3 &     74.4 &     66.5 & \bf 77.2 & \bf 75.9 & \bf 75.5\\
\mourmethod{} (G) & \bf 86.3 & \bf 73.2 &     77.9 & \bf 79.0 &     76.5 &     80.3 & \bf 80.4 & \bf 70.8 & \bf 76.7 &     62.9 &     74.2 & \bf 74.5 & \bf 66.6 &     76.5 &     75.7 &     75.4\\
\midrule
\multicolumn{17}{l}{\emph{Translate-train (models fine-tune on English training data plus translations in all target languages)}} \\
\midrule
XLM & 85.0  &76.5 &79.3 & 80.3 & 78.1 & 80.3&80.2& 72.3&78.1& 70.9&75.5&74.7 &63.2&76.6&78.6& 76.6  \\
\mourmethod{} (D)&      85.9& \bf 76.9  & \bf 79.9 &     80.7  & \bf 79.5 & \bf 81.6 &     80.9 &     74.2 & \bf 78.7 & \bf 71.8 &     76.9 &     76.9 & \bf 65.8 &     79.1 & \bf 80.0 & 77.9 \\
\mourmethod{} (G)&  \bf 86.3&     76.7  &     79.7 & \bf 80.8  &     79.7 &     81.6 & \bf 82.0 & \bf 74.6 &     78.6 &     70.8 & \bf 77.4 & \bf 77.1 &     65.3 & \bf 79.2 &    79.3  & \bf 77.9 \\
\midrule
\multicolumn{17}{l}{\emph{Translate-train (models fine-tune on English training data plus translations in all target languages)}} \\
\midrule
XLM       & 85.0  & 77.6 & 80.9 & 80.3 & 79.1 & 81.3 & 80.8 & 72.9 & 78.3 & 72.8 & 76.0 & 75.6 & 68.5 & 78.5 & 79.5 & 77.8  \\
mT5-Small & 69.5  & 63.7 & 67.5 & 65.7 & 66.4 & 67.5 & 67.3 & 61.9 & 66.4 & 59.6 & 63.9 & 63.5 & 60.4 & 63.3 & 64.5 & 64.7 \\
mT5-Base & 82.0 & 74.4 & 78.5 & 77.7 & 78.1 & 79.1 & 77.9 & 72.2 & 76.5 & 71.5 & 75.0 & 74.8 & 70.4 & 74.5 & 76.0   & 75.9 \\
\mourmethod{} (D)&  \bf 87.3 & \bf 78.3 &     82.7 & \bf 83.1 &     82.2 &     83.8 &     83.3 & \bf 77.3 &     81.3 &     73.1 & \bf 80.3 & \bf 79.9 &     71.2 &     81.3 & \bf 81.8 &     80.5 \\
\mourmethod{} (G)&      87.2 &     78.3 & \bf 83.3 &     82.7 & \bf 82.3 & \bf 84.0 & \bf 83.6 &     77.1 & \bf 81.4 & \bf 74.5 &     79.8 &     79.6 & \bf 71.3 & \bf 81.6 &     81.6 & \bf 80.6 \\
\bottomrule
\end{tabular}}
\caption{XNLI accuracy scores for each language.}
\end{table*}
%%%%%%%%%%%%%%%%%%%%%%%%%%%%%%%%%%%%%%%%%%%%%%%%%%%%%%%%%%%%%%%%%%%%%%%%%%%%%%%%%%%%%%

%%%%%%%%%%%%%%%%%%%%%%%%%%%%%%%%%%%%%%%%%%%%%%%%%%%%%%%%%%%%%%%%%%%%%%%%%%%%%%%%%%%%%%
% \begin{figure*}[t]
% \begin{center}
% 	\includegraphics[width=0.95\textwidth]{graph/flores.pdf}
% 	\caption{Evaluation results of our multilingual model on all translation directions on the FLORES-101 devtest set, where our model consists of 12 encoder and 12 decoder layers with a hidden size of 768. We fine-tune the multilingual encoder-decoder pre-trained model \mourmethod{} on the large-scale dataset.
% 	The language $x$ in the $i$-th row and language $y$ in the $j$-th column denotes the translation direction from the language $x$ to language $y$. For example, the cell of the $1$-st row (af) and the $3$-nd column (ar) represents the result of the translation direction af$\to$ar. The table shows the results of all translation directions of 102 languages.}
% 	\label{flores_all}
% \end{center}
% \end{figure*}
%%%%%%%%%%%%%%%%%%%%%%%%%%%%%%%%%%%%%%%%%%%%%%%%%%%%%%%%%%%%%%%%%%%%%%%%%%%%%%%%%%%%%%

\section{Weight Sharing}
%%%%%%%%%%%%%%%%%%%%%%%%%%%%%%%%%%%%%%%%%%%%%%%%%%%%%%%%%%%%%%%%%%%%%%%%%%%%%%%%%%%%%%
\begin{table}[t]
\centering
\resizebox{1.0\columnwidth}{!}{
\begin{tabular}{c|c|c|c|c}
\toprule
\bf ID      & \bf \#Params   & \bf Strategy   &  \makecell[c]{\textbf{Xsum} \\ RG-1/RG-2/RG-L} & \makecell[c]{\textbf{WMT16 En-Ro} \\ En$\to$Ro/Ro$\to$En}    \\
\midrule
{\large{\ding{172}}} & 390M &$\theta_{\mathcal{G}} =\theta_{\mathcal{D}}$& 43.26/19.82/35.02     &  37.4/37.2\\
{\large{\ding{173}}} & 430M &$\theta_{\mathcal{G}}\neq \theta_{\mathcal{D}}$& \bf 45.36/21.98/36.84 &\bf 38.3/38.0 \\ 

\bottomrule
\end{tabular}
}
\caption{Evaluation results with different weight sharing strategies on the test set of the Xsum summarization task and WMT16 En-Ro translation task. Both generator decoder $\theta_{\mathcal{G}}$ and discriminator decoder $\theta_{\mathcal{D}}$ have 12 layers in Experiment {\large{\ding{173}}} by sharing decoder parameters.
}
\label{weight_sharing}
\vspace{-10pt}
\end{table}
%%%%%%%%%%%%%%%%%%%%%%%%%%%%%%%%%%%%%%%%%%%%%%%%%%%%%%%%%%%%%%%%%%%%%%%%%%%%%%%%%%%%%%

Our pre-trained model includes the discriminator $(\mathcal{D}: \{\theta_{\mathcal{E}},\theta_{\mathcal{D}}\})$ and generator $(\mathcal{G}: \{\theta_{\mathcal{E}},\theta_{\mathcal{G}}\})$. We can use a 12-layer generator decoder $\theta_{\mathcal{G}}$ and a 4-layer tiny discriminator decoder $\theta_{\mathcal{D}}$ for \gtask{}. We propose a weight sharing strategy to improve the model efficiency of the pre-training by sharing weights among the generator and decoder ($\theta_{\mathcal{D}}=\theta_{\mathcal{G}}$) by setting the discriminator generator and generator decoder as the same size (both 12 layers). Table \ref{weight_sharing} lists the results of different weight sharing strategies. It turns out the sharing decoder setting performs worse than not sharing. It is reasonable since the generator decoder is used for sequence generation whereas the discriminator decoder is a classifier.
